# Supplementary material for: Emergence of dynamic vortex glasses in disordered polar active fluids
Source: arXiv:2002.12893 ancillary file (2020-09-07)
Supplement: Supplementary file 1 [file SI.pdf]

# Meandering flows and dynamical vortex glasses in disordered polar active matter

## SUPPLEMENTARY INFORMATION

Amélie Chardac[1], Suraj Shankar[2], M. Cristina Marchetti[3], and Denis Bartolo[1]
[1] *Univ. Lyon, ENS de Lyon, Univ. Claude Bernard, CNRS, Laboratoire de Physique, F-69342, Lyon, France*
[2] *Department of Physics, Harvard University, Cambridge, MA 02318, USA and*
[3] *Department of Physics, University of California Santa Barbara, Santa Barbara, CA 93106, USA*
(Dated: August 13, 2020)

## CONTENTS

I. Eulerian fields from Lagrangian trajectories 2

II. Edwards–Anderson order parameter and relaxation times 3

III. Detection of the topological defects 4

IV. Multiplicity of the stationnary meandering flows 5

V. Flocking through periodic lattices 7

VI. Toner-Tu equations with quenched disorder 8
A. Linearized theory of the ordered-phase fluctuations 8
B. Long range polar order in disordered media: comparison with numerical and theoretical studies 9

VII. Flocking through quenched disorder beyond the spin-wave approximation: Mapping to random XY model 9

VIII. Disorder-induced vortex creation and onset of meandering flows: a Kosterlitz-Thouless style argument 11

IX. Description of the Supplementary Videos 12

References 13

## I. EULERIAN FIELDS FROM LAGRANGIAN TRAJECTORIES

All measurements are systematically repeated three times for different initial conditions and same disorder configuration. If not specified otherwise, we measure all quantities reported in the main text after the ensemble of rollers has reached its stationary state.

**Lagrangian trajectories.** As explained in the Methods section, we detect the position of all the rollers with a sub-pixel accuracy using the algorithm introduced by Lu et al in [1]. We then reconstruct their trajectories over the whole 3 mm wide circular chambers using the Crocker and Grier algorithm [2] with the MATLAB routine available at [3].

We define the individual roller velocities from their displacements over two subsequent frames (time interval: $\delta t = 5.3\,\mathrm{ms}$): $\mathbf{v}_i(t) = \mathbf{r}_i(t+\delta t) - \mathbf{r}_i(t)$, where $\mathbf{r}_i(t)$ and $\mathbf{v}_i(t)$ are respectively the position and velocity of particule $i$ at time $t$. The accuracy of the position measurements is of the order of $0.1\,\mu\mathrm{m}$, inducing an accuracy of the order of $40\,\mu\mathrm{m/s}$ for individual speed measurements. When powered with an electric field $\mathbf{E}$ of magnitude 120 V, all colloids roll at a constant speed

$$v_0 = 0.80 \pm 0.04\,\mathrm{mm/s}. \tag{S1}$$

In addition, when isolated, their direction of motion freely diffuses on the unit circle with a rotational diffusivity

$$D_r = 2.2 \pm 0.1\,\mathrm{s}^{-1}, \tag{S2}$$

where $D_r$ is defined as the exponential decorrelation rate of the velocity orientation in an isotropic phase.

**Eulerian fields.** Building on these Lagrangian measurements, we reconstruct the instantaneous Eulerian velocity fields $\mathbf{v}(\mathbf{r}, t)$ as follows. We average the instantaneous roller velocities in $76.4\,\mu\mathrm{m} \times 76.4\,\mu\mathrm{m}$ binning windows arranged on a square lattice with a lattice spacing of $15.3\,\mu\mathrm{m}$. Given the roller density, each PIV window typically averages the velocity of 25 rollers. We systematically checked that none of our results crucially depends on the specific choice of the size of the binning windows. The polarization and overlap fields are computed with the same spatial resolution from $\mathbf{v}(\mathbf{r}, t)$.

To compute the polarization order parameter from the instantaneous velocity field, we first average the radial and azimuthal components of the polarization field $\boldsymbol{p}(\mathbf{r}) \equiv \langle \hat{\mathbf{v}}(\mathbf{r},\mathrm{t})\rangle_{\mathrm{t}}$ over square boxes of size $\ell$. We then compute the spatial average: $\boldsymbol{p}_B \equiv (\langle p_r(\mathbf{r})\rangle_{\mathbf{r}}, \langle p_\theta(\mathbf{r})\rangle_{\mathbf{r}})$, in each box $B$. Finally, $\mathcal{P}(\ell)$ corresponds to the norm of $\boldsymbol{p}_B$ averaged over all boxes $B$.

## II. EDWARDS–ANDERSON ORDER PARAMETER AND RELAXATION TIMES

The Edwards–Anderson parameter quantifies the time persistence of the emergent flows. It is defined in terms of the long-time behavior of the two-time velocity correlation function $\mathcal{Q}(T) = \langle \hat{\mathbf{v}}(\mathbf{r}, t) \cdot \hat{\mathbf{v}}(\mathbf{r}, t+T)\rangle_{\mathbf{r},t}$, as $\mathcal{Q}_{\rm EA} = \langle \hat{\mathbf{v}}(\mathbf{r}, t) \cdot \hat{\mathbf{v}}(\mathbf{r}, t+T)\rangle_{\mathbf{r},t,T\to\infty}$. As shown in Fig. S1, velocity correlations decay to a plateau value in a time smaller than 4 seconds (the minimal duration of our experiments). We therefore define $\mathcal{Q}_{\rm EA} \equiv \mathcal{Q}(T = 4\,{\rm s})$.

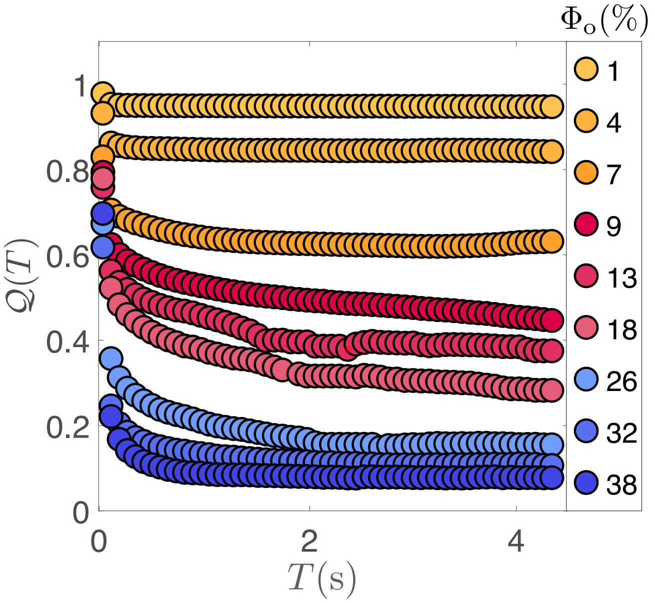


FIG. S1. **Velocity correlation**. Plot of two-time correlation function $\mathcal{Q}(T) = \langle \hat{\mathbf{v}}(\mathbf{r}, t) \cdot \hat{\mathbf{v}}(\mathbf{r}, t+T)\rangle_{\mathbf{r},t}$ as a function of the lag time $T$. The decorrelation time of the orientation field is smaller than the duration of our measurements.

## III. DETECTION OF THE TOPOLOGICAL DEFECTS

The topological defects are singularities of the orientation field $\hat{\mathbf{v}}(\mathbf{r},t) \equiv (\cos\theta(\mathbf{r},t), \sin\theta(\mathbf{r},t))$. We can readily visualize their instantaneous position inspecting the Schlieren texture obtained from the map of $\theta(\mathbf{r},t)$, see Figs. S2a and S2c. We detect the position of all the defects, by computing the winding number $w_{ij}$ of the flow orientation at each point $(i,j)$ on the PIV grid as sketched in Fig. S2b. In practice, $w_{ij}$ is the sum of the differences between the adjacent $\theta$ angles along the contour defined by the 8 nearest neighbors of $(i,j)$.

In the absence of singularity $w_{ij}$ vanishes. Conversely, at a singular point, $w_{ij}$ takes a finite and quantized value that defines the defect charge $q = w_{ij}/(2\pi)$. We applied the same procedure to detect the defects of the time-averaged polarization field $\mathbf{p}(\mathbf{r})$.

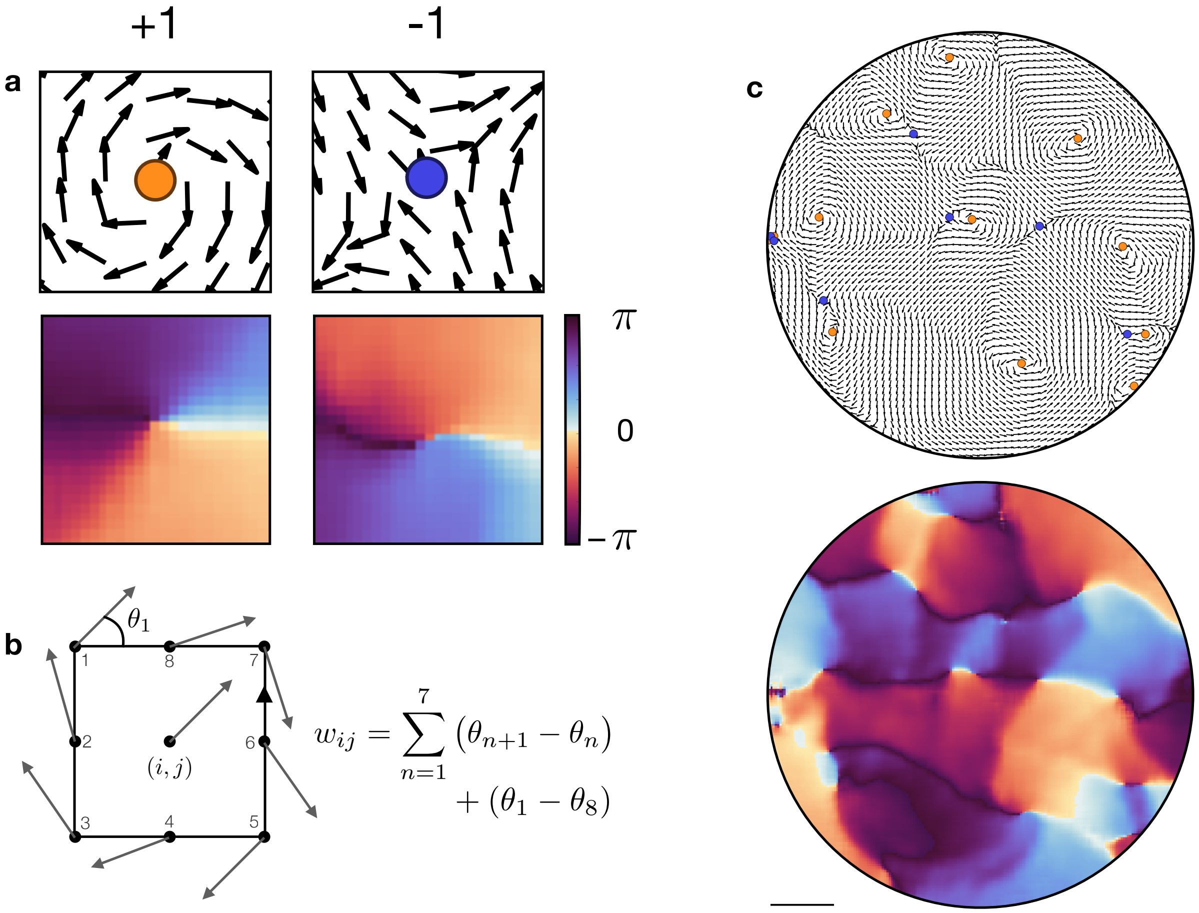


FIG. S2. **Detection of the topological defects**. **a**, Correspondence between the Schlieren pattern and the polarization field in the vicinity of +1 and −1 defects. **b**, Calculation of the local winding $w_{ij}$ of the polarization field. **c**, Schlieren pattern of the polarization field in the meander phase ($\Phi_o = 9\,\%$) and corresponding polarization field with detected topological defects. Scale bar: 0.5 mm.

In order to evaluate the accuracy of our detection algorithm, we rely on the conservation of topological charge in the circular chamber. As we only detect defects of charges +1 or −1, the total topological charge of $\hat{\mathbf{v}}(\mathbf{r},t)$ is given by the difference of the number of defects of opposite charges at time $t$: $\mathcal{C}(t) = \mathcal{N}_+(t) - \mathcal{N}_-(t)$. In the vortex phase the total charge hardly fluctuates around: $\mathcal{C}(t) = 1$, as the charge is trivially supported by a single +1 defect at the center of the chamber. In the meander phase, although a number of defects coexist, the instantaneous charge distribution is a Gaussian that remains narrowly peaked around $C(t) = 0.8$, see Fig. S3. Similarly, the distribution of charge of the $\boldsymbol{p}(\mathbf{r})$ field computed in each replica $(\mathrm{P}(\mathcal{C}_\alpha))$ peaks at $C_\alpha = 1.4$. The errorbars on our defect number measurement are therefore defined as the standard deviation of $\mathcal{C}(t)$ and $\mathcal{C}_\alpha$.

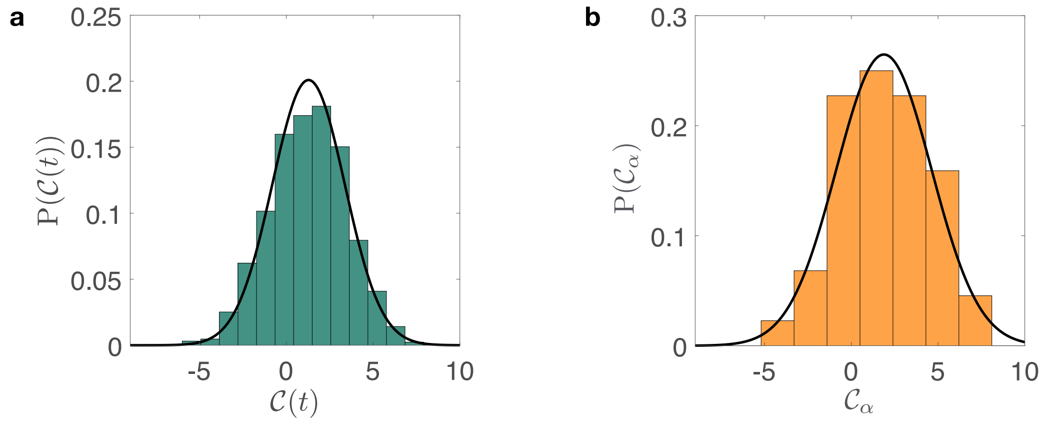


FIG. S3. **Distribution of the topological charge**. **a**, Probability distribution function of the instantaneous topological charge $\mathcal{C}(t)$ of the $\hat{\mathbf{v}}(\mathbf{r},t)$ field measured in the meander phase ($\Phi_o = 15\,\%$). Dark line: Gaussian best fit. Average: $\langle\mathcal{C}(t)\rangle_t = 0.8$, standard deviation $\langle\Delta\mathcal{C}^2(t)\rangle_t^{1/2} = 2.2 \ll \langle\mathcal{N}(t)\rangle_t$. **b**, Probability distribution of the topological charge of the polarization field measured in fifty replica of a meander phase ($\Phi_o = 15\,\%$). Dark line: Gaussian best fit. Average: $\langle\mathcal{C}_\alpha\rangle_\alpha = 1.4$, standard deviation $\langle\Delta\mathcal{C}_\alpha^2\rangle_\alpha^{1/2} = 2.3 \ll \langle\mathcal{N}_\alpha\rangle_\alpha$.

## IV. MULTIPLICITY OF THE STATIONNARY MEANDERING FLOWS

We detail the method to estimate the number of nonequivalent steady states among all the replicated meanders. The fourty-two overlap fields showed in Fig. S5 clearly indicate that the local flows are either parallel or antiparallel in each pair of replicas. In order to determine the fraction of space where meanders flow in the same direction, we first plot the local overlap $q_{\alpha\beta}(\mathbf{r}) = \boldsymbol{p}_\alpha(\mathbf{r})\cdot\boldsymbol{p}_\beta(\mathbf{r})$ averaged over all pairs of replicas $(\alpha,\beta)$ (with $\alpha\neq\beta$). In agreement with our qualitative observation, the distribution $\mathrm{P}(\mathrm{q}_{\alpha\beta}(\mathbf{r}))$ is asymmetric but sharply peaked at $\pm1$, Fig. S4a. In order to single out the contributions to $P(q_{\alpha\beta}(\mathbf{r}))$ coming from the regions of space where disorder prescribes the flow orientation, we proceed as follows. We first consider the negative part of the distribution, symmetrize it and substract this symmetric function from $\mathrm{P}(\mathrm{q}_{\alpha\beta}(\mathbf{r}))$ as sketched in Fig. S4. As a matter of fact, if the obstacles focused the flows along preferred channels without specifying its orientation, the overlap distribution would be symmetric and peaked on $\pm1$. We can therefore measure the fraction of space where disorder fully prescribes the orientation of the flows by computing the integral of the curve plotted in Fig. S4c. This area fraction is equal to 0.46 in our experiments.

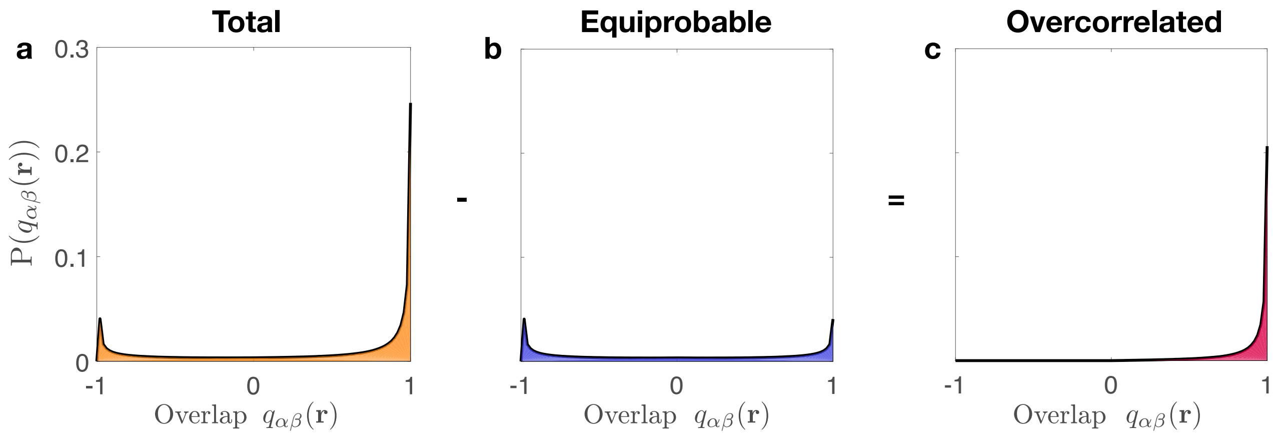


FIG. S4. **Decomposition of the overlap distribution**. **a**, Overlap distribution over all replicas: $\mathrm{P}(\mathrm{q}_{\alpha\beta}(\mathbf{r}))$. **b**, Symmetrization of the negative part of $\mathrm{P}(\mathrm{q}_{\alpha\beta}(\mathbf{r}))$. **c**, Difference between the overlap distribution and the symmetrization of its negative part.

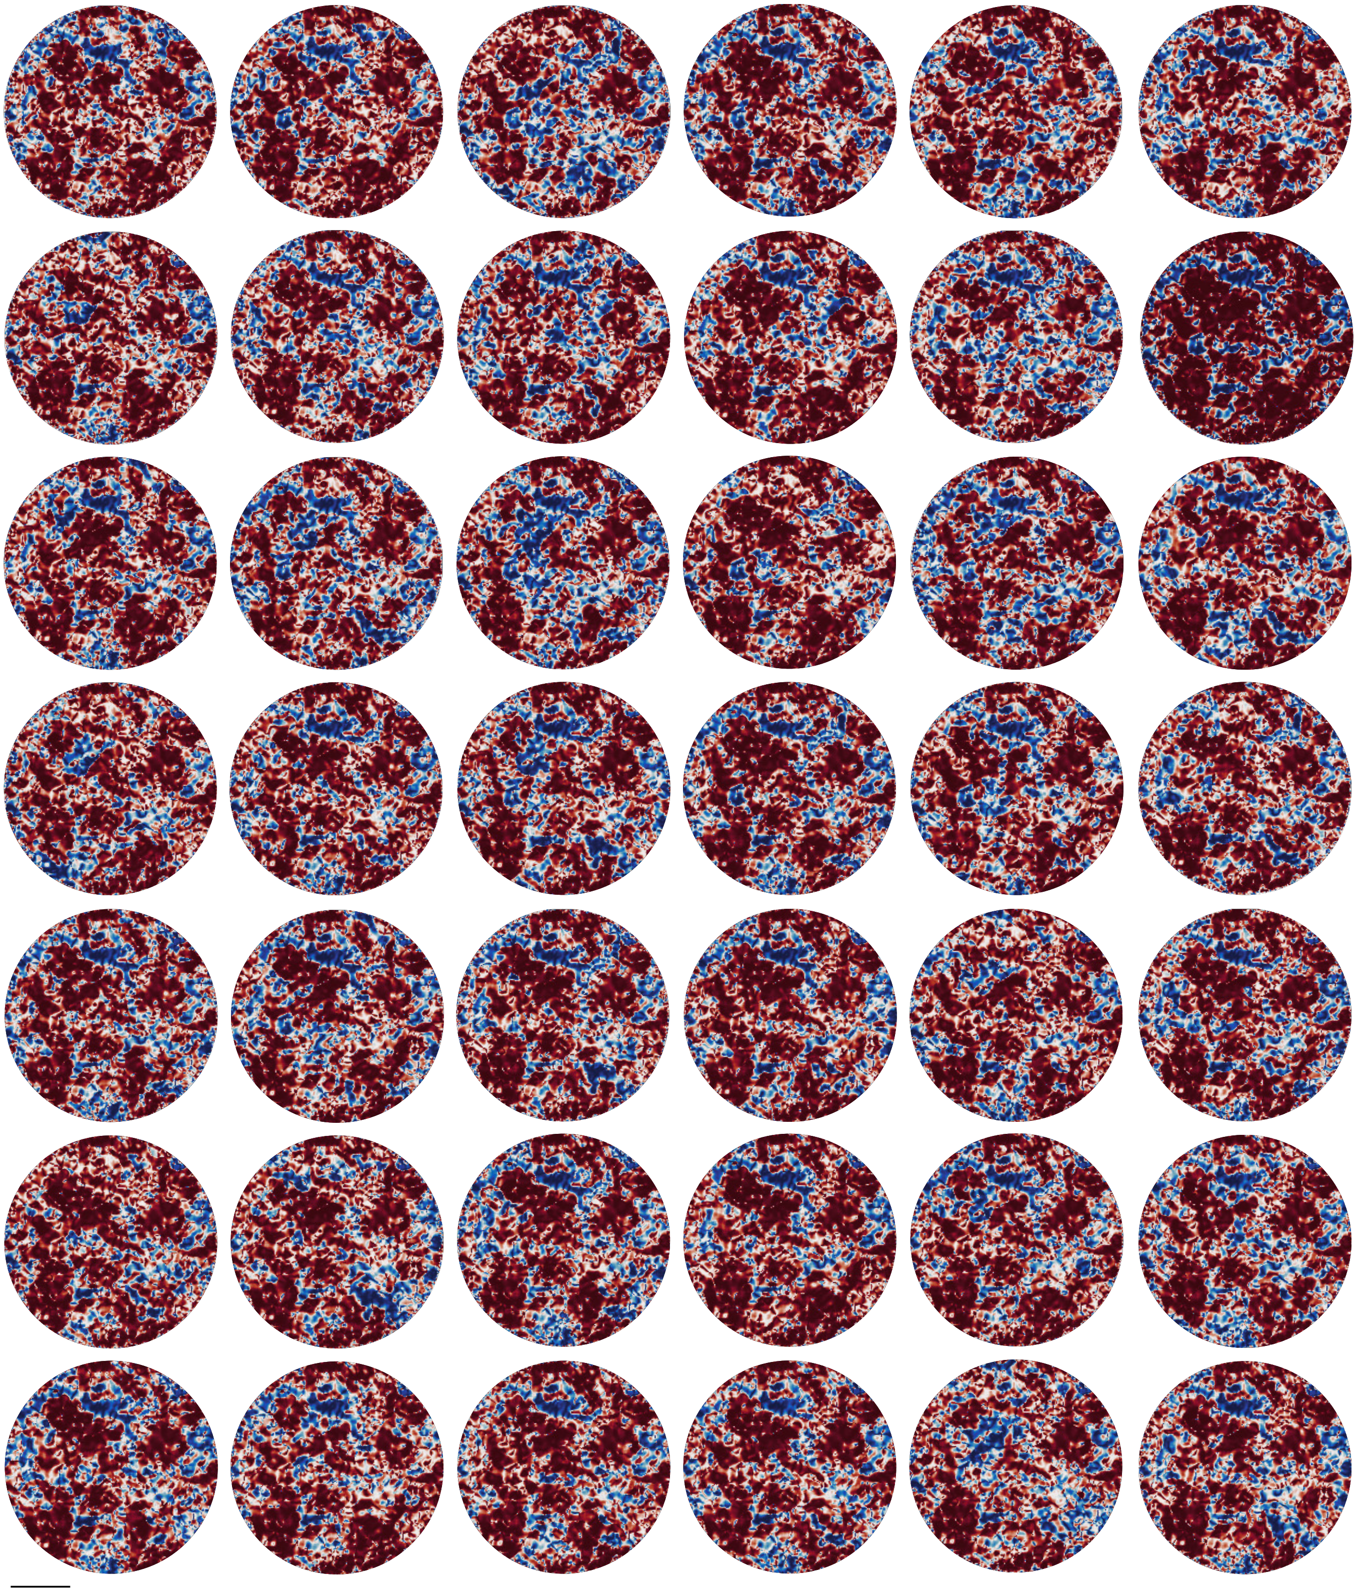

FIG. S5. **Polarization overlap**. We show the overlap between one replica and all the others. The 42 maps are all different thereby revealing the multiplicity of the steady meandering flows. They also indicate that the meanders locally flow either along the same or the opposite direction. Scale bar: 1 mm. Colormap: red for $q_{\alpha\beta} = 1$; blue for $q_{\alpha\beta} = -1$ and white for $q_{\alpha\beta} = 0$.

## V. FLOCKING THROUGH PERIODIC LATTICES

We report below a series of experiments conducted in triangular lattices of obstacles, see Fig. S6a and Supplementary Video 7. The phase behavior of the rollers is markedly different than in disordered systems. Plotting the polarization and Edwards–Anderson order parameters in Fig. S6b, we find that $\mathcal{P}$ and $\mathcal{Q}_{\rm EA}$ vanish at the same obstacle fraction: no meander phase is observed in periodic geometries. Global polar order survives to higher obstacle fractions and is directly suppressed to form a gas phase at high $\Phi_{\rm o}$, as further confirmed by the comparisons of the $\mathcal{N}(\Phi_{\rm o})$ plots. This essential distinction with disordered systems establishes that the emergence of meandering flows stems from the spatial heterogeneities of the obstacle patterns.

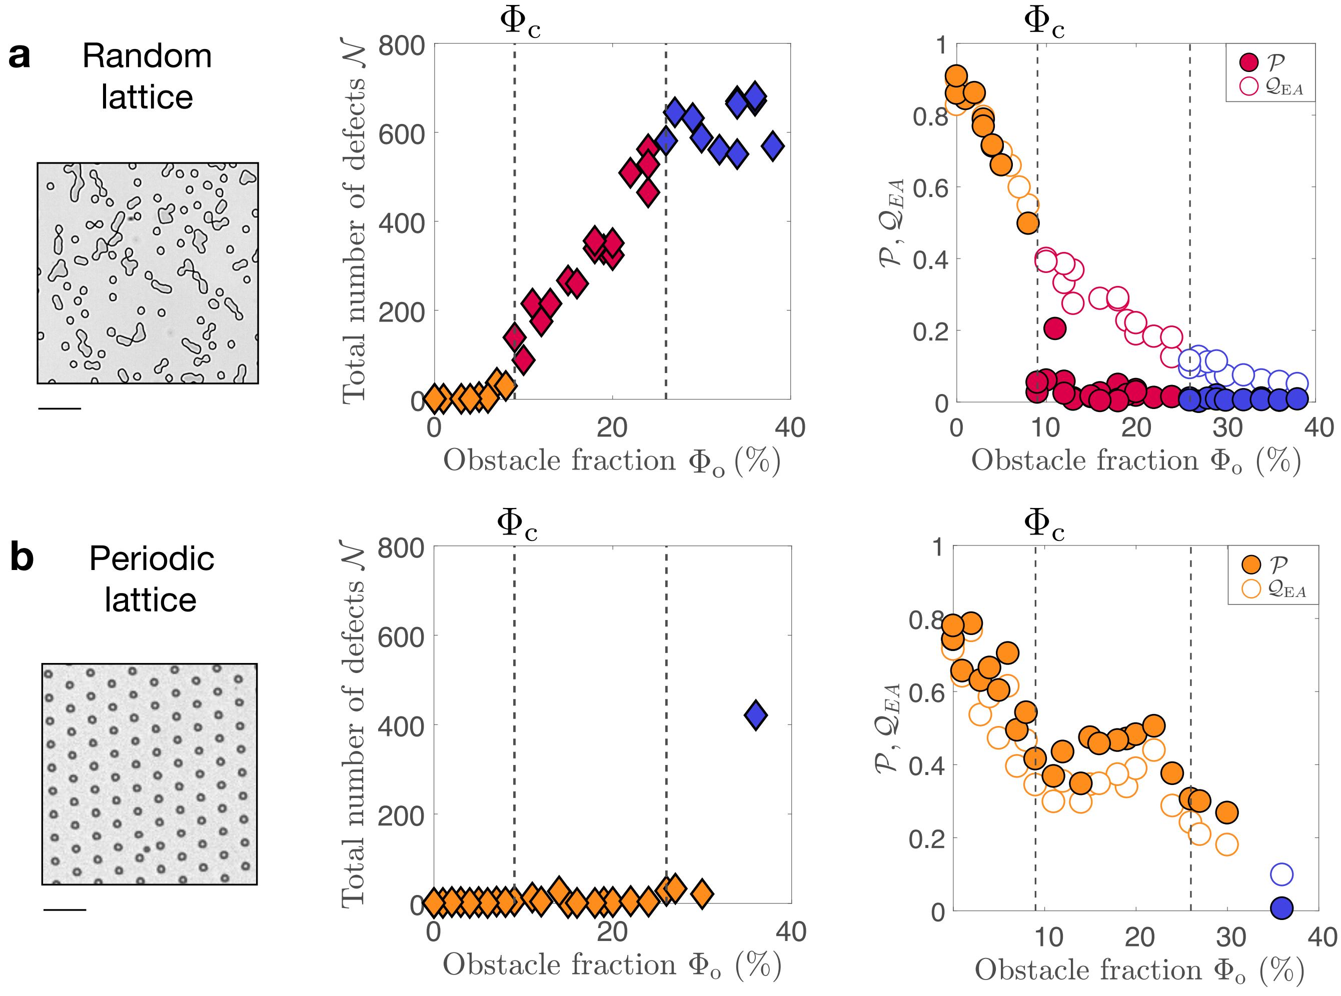


FIG. S6. **Flocking through periodic lattices**. **a**, Close-up picture of a random lattice of obstacles (scale bar: 50 $\mu$m, obstacle fraction $\Phi_{\rm o} = 15\,\%$) and reminder of the results detailed in the main text. Variations of the total number of topological defects with the obstacle fraction and plot of the polarization and Edwards-Anderson order parameters distinguishing the gas, meander and vortex phases. **b**, Close-up picture of a triangular lattice of obstacles (scale bar: 50 $\mu$m, obstacle fraction $\Phi_{\rm o} = 15\,\%$). The meander phase is suppressed. The number of defects jumps from 1 to a finite value in the gas phase upon increasing $\Phi_{\rm o}$. Similarly, $\mathcal{P}$ and $\mathcal{Q}_{\rm EA}$ both vanishes at $\Phi_{\rm o} = 38\%$ thereby revealing a direct transition from a polar liquid to an active gas phase.

## VI. TONER-TU EQUATIONS WITH QUENCHED DISORDER

In order to theoretically account for our experimental findings, we start with a minimal version of Toner–Tu hydrodynamics for an active polar fluid in 2D [4, 5]. This simplified model proved to yield an accurate description of the macroscopic flows of Quincke-roller fluids in homogeneous media [6]. While there are multiple ways of including quenched disorder, here we only consider random *potential* (scalar) disorder arising from static isotropic obstacles. The influence of random *field* (vector) disorder is markedly different and has recently been theoretically analyzed in Refs. [7, 8]. Since the obstacle-roller interaction is isotropic, and the obstacles are otherwise featureless, we follow the arguments given in Ref. [9] to get

$$\partial_t\rho + \boldsymbol{\nabla}\cdot(\rho\mathbf{v}) = 0\ , \tag{S3}$$

$$\partial_t\mathbf{v} + \lambda\mathbf{v}\cdot\boldsymbol{\nabla}\mathbf{v} = \left(a_2 - a_4|\mathbf{v}|^2\right)\mathbf{v} + K\nabla^2\mathbf{v} - \beta\boldsymbol{\nabla}\rho - \beta_{\rm o}\boldsymbol{\nabla}\phi_{\rm o}\ , \tag{S4}$$

where the number density $\rho$ simply obeys the continuity equation and $\mathbf{v}$ is the fluid velocity. The coefficients $a_2, a_4 > 0$ allow for a mean field polar ordered state ($\langle\mathbf{v}\rangle \neq \mathbf{0}$), the elastic constant $K$ penalizes flow distortions, $\beta$ is an effective inverse compressibility modulus, and the active kinetic coefficient $\lambda$ controls advection. Quenched disorder enters through a static random potential with a positive coupling $\beta_{\rm o}$ and has correlations set by the mean obstacle density $\Phi_{\rm o}$,

$$\overline{\phi_{\rm o}(\mathbf{r})} = \Phi_{\rm o}\ ,\quad \overline{\left(\phi_{\rm o}(\mathbf{r}) - \Phi_{\rm o}\right)\left(\phi_{\rm o}(\mathbf{r}') - \Phi_{\rm o}\right)} = \Phi_{\rm o}\delta(\mathbf{r}-\mathbf{r}')\ . \tag{S5}$$

Writing $\mathbf{v} = v(\cos\theta, \sin\theta)$, and using the shorthand notation $\partial_{||} \equiv \hat{\mathbf{v}}\cdot\boldsymbol{\nabla} = \cos\theta\partial_x + \sin\theta\partial_y$ and $\partial_\perp \equiv \hat{\mathbf{z}}\cdot(\hat{\mathbf{v}}\times\boldsymbol{\nabla}) = \cos\theta\partial_y - \sin\theta\partial_x$, Toner–Tu hydrodynamics reduces to

$$\partial_t\rho + \partial_{||}(\rho v) + \rho v\partial_\perp\theta = 0\ , \tag{S6}$$

$$\partial_t\theta + \lambda v\partial_{||}\theta = K\nabla^2\theta + \frac{2K}{v}\boldsymbol{\nabla}v\cdot\boldsymbol{\nabla}\theta - \frac{\beta}{v}\partial_\perp\rho - \frac{\beta_{\rm o}}{v}\partial_\perp\phi_{\rm o}\ , \tag{S7}$$

$$\partial_t v + \lambda v\partial_{||}v = \left(a_2 - a_4v^2\right)v + K\nabla^2 v - Kv|\boldsymbol{\nabla}\theta|^2 - \beta\partial_{||}\rho - \beta_{\rm o}\partial_{||}\phi_{\rm o}\ . \tag{S8}$$

### A. Linearized theory of the ordered-phase fluctuations

The first noticable consequence of disorder is the monotonic decay of the polarization order parameter with $\Phi_{\rm o}$ in the vortex phase. We can account for this behavior considering the linear fluctuations caused by disorder on homogeneous polar flows. Linearizing about the polar ordered state, we have $\rho = \rho_0 + \delta\rho$ and $\mathbf{v} = v_0(\hat{\mathbf{x}} + \delta\theta\hat{\mathbf{y}})$, where $v_0 = \sqrt{a_2/a_4}$. Ignoring the rapidly relaxing amplitude fluctuations ($\delta v = 0$) deep in the ordered state, Eqs. S6 and S7 reduce to

$$\partial_t\rho + v_0\partial_x\delta\rho + \rho_0 v_0\partial_y\delta\theta = 0\ , \tag{S9}$$

$$\partial_t\delta\theta + c_{||}\partial_x\delta\theta = K\nabla^2\delta\theta - \frac{c_\perp^2}{\rho_0 v_0}\partial_y\delta\rho - \frac{\beta_{\rm o}}{v_0}\partial_y\phi_{\rm o}\ , \tag{S10}$$

where we have introduced the longitudinal ($c_{||} = \lambda v_0$) and transverse ($c_\perp = \sqrt{\beta\rho_0}$) sound speeds. Following ref. [9], we Fourier transform in space ($\Phi_{\mathbf{q}} = \int \mathrm{d}\mathbf{r}\ e^{-i\mathbf{q}\cdot\mathbf{r}}\Phi(\mathbf{r})$), and set the time derivatives to zero at steady-state to compute the power spectrum of the orientational fluctuations averaged over disorder realizations:

$$\overline{|\delta\theta_{\mathbf{q}}|^2} = \frac{\beta_{\rm o}^2\Phi_{\rm o}\sin^2 2\psi}{4\left[(c_{||}v_0\cos^2\psi - c_\perp^2\sin^2\psi)^2 + v_0^2q^2\cos^2\psi K^2\right]}\ , \tag{S11}$$

where $q = |\mathbf{q}|$, and $\psi$ is the angle between $\mathbf{q}$ and the $x$-axis (direction of mean order). The density correlator is similarly given by $\overline{|\delta\rho_{\mathbf{q}}|^2} = (\rho_0 q_y^2/q_x^2)\overline{|\delta\theta_{\mathbf{q}}|^2}$. We note that $c_{||}v_0 > 0$ for the Quincke-roller fluid [6], due to which the correlator is highly anisotropic with a singular scaling at $\psi = \pm\psi_c$, where $\tan\psi_c = \sqrt{c_{||}v_0}/c_\perp$ [7, 8]. As a result, $\overline{|\delta\theta_{\mathbf{q}}|^2}$ is finite as $q \to 0$ for $\psi \neq \pm\psi_c$, while right at $\psi = \pm\psi_c$, we have $\overline{|\delta\theta_{\mathbf{q}}|^2} \sim q^{-2}$ as $q \to 0$. Going back to real space, we then find that quenched disorder cause finite orientational fluctations. More quantitatively we find that

$$\overline{\delta\theta(\mathbf{r})^2} \approx \int\frac{\mathrm{d}q}{2\pi}q\int\frac{\mathrm{d}\delta\psi}{2\pi}\frac{\beta_{\rm o}^2\Phi_{\rm o}\sin^2 2\psi_c}{4\left[4c_{||}c_\perp^2v_0\delta\psi^2 + v_0^2K^2\cos^2\psi_c q^2\right]} = \frac{\beta_{\rm o}^2\Phi_{\rm o}\sin^2 2\psi_c}{16Kv_0c_\perp\sqrt{c_{||}v_0}|\cos\psi_c|}\int_0^\Lambda\frac{\mathrm{d}q}{2\pi} < \infty\ . \tag{S12}$$

As a consequence, the velocity fluctuations remain finite on large scales thereby allowing for genuine *long-ranged order* to survive to quenched disorder. In addition, the fact that $\overline{\delta\theta(\mathbf{r})^2} \propto \Phi_{\rm o}$ implies that the mean polarization decreases linearly with increasing obstacle density, in agreement with our experimental observations (see Fig. 2 in the main text).

### B. Long range polar order in disordered media: comparison with numerical and theoretical studies

As mentioned previously, it is important to distinguish between *scalar* and *vectorial* disorder. The former is relevant when the disorder is featureless and characterized by locally isotropic impurities, and is akin to scalar potential disorder in equilibrium systems. The latter on the other hand involves locally *anisotropic* impurities and are hence vectorial in nature, akin to random field disorder in equilibrium systems. Most previous active-matter work has focused on vectorial disorder, by contrast very little is known about the much weaker scalar counterpart.

Previous numerical [10] and theoretical [7, 8] work has looked at the impact of quenched vectorial disorder on Toner–Tu polar active fluids, showing that the long-range order present in the clean system is immediately lost, giving way to only quasi-long range order. More recently, Maitra analyzed the impact of weak vectorial disorder on active suspensions in contact with a substrate [11]. In this case, long-ranged polar order can survive for finite disorder due to the incompressibility of the suspending fluid. We stress that the Quincke rollers, although dispersed in an incompressible fluid, are accurately described by the conventional Toner–Tu hydrodynamics due to the screening of the far-field hydrodynamic interactions and the weak confinement of the fluid flows by the conducting electrodes, see [6] and associated SI. In addition, all of these previous works have only addressed the consequences of vectorial disorder, which as such does not describe the system at hand. As a result, there is no possible contradiction with our work.

Some earlier numerical studies considered the case of quenched scalar disorder [12]. In this work Chepizhko and Peruani showed that long-ranged polar order can survive in 2D active fluids upto a finite disorder threshold. Their conclusion was based on numerical simulations of a Vicsek model with self-propelled point particles that align with their neighbours and repel from isotropic point obstacles. This result is consistent with our theoretical and experimental findings. It is however worth noting, that unlike in our experiments the authors of [12] also found a regime with quasi long range order. Having in mind living systems, the authors simulated non-pairwise additive interactions between the particle and the obstacles and between the active- particles. This crucial difference with our experiments could explain the apparent discrepency.

## VII. FLOCKING THROUGH QUENCHED DISORDER BEYOND THE SPIN-WAVE APPROXIMATION: MAPPING TO RANDOM XY MODEL

Deep in the polar ordered state, we can neglect amplitude fluctuations and fix $|\mathbf{v}| = v_0$. For the time being, we shall also neglect density fluctuations and set $\rho = \rho_0$, a constant as we are primarily interested in elucidating the effect of quenched disorder on distorting the flow. A more sophisticated analysis involving the density and nonlinear fluctuations is left for future work. From Eqs. S6, S7, to lowest order in gradients, we get

$$\partial_\perp \theta = 0 \ , \quad \lambda v_0 \partial_{||}\theta \simeq -\frac{\beta_{\rm o}}{v_0}\partial_\perp \phi_{\rm o} \ . \tag{S13}$$

The physical content of these equations is that the flow streamlines cannot cross or form caustics ($\boldsymbol{\nabla}\cdot\hat{\mathbf{v}} = \partial_\perp\theta = 0$) and that maintaining a bent streamline ($\partial_{||}\theta \neq 0$) requires an effective centrifugal force that is provided here by the random pressure gradient generated by the spatial distribution of obstacles. Hence, as a result of balancing the random pressure fluxes due to disorder with the convective flux due to distortions in the polar flow, we obtain an implicit condition that solves Eq. S13,

$$\boldsymbol{\nabla}\theta = -\frac{\beta_{\rm o}}{\lambda v_0^2}\boldsymbol{\epsilon}\cdot\mathbb{P}\boldsymbol{\nabla}\Phi_o \equiv \mathcal{A} \ , \tag{S14}$$

where $\boldsymbol{\epsilon}$ is the 2D Levi-Civita tensor and $\mathbb{P} = \mathbf{1} - \hat{\mathbf{v}}\hat{\mathbf{v}}$ is a transverse projection operator. Eq. S14 has a clear physical meaning: the static obstacles create pressure gradients that balance with convective fluxes to imprint a quenched distribution of preferred orientational, viz. phase distortions. In other words, the obstacles generate a random gauge field $\mathcal{A}$, with an associated charge density $Q = \hat{\mathbf{z}}\cdot(\boldsymbol{\nabla}\times\mathcal{A})$ quenched in the background. The polar fluid then navigates these obstacles by generating meandering flows that match the required phase distortion, primarily penalized by orientational elasticity ($K$). The competition between the random gauge field and orientational elasticity

underlies the essential physics of meandering flows. Note the crucial role of activity in realizing the effective gauge field $\mathcal{A}$ in a nonperturbative fashion as $\mathcal{A}$ diverges for $v_0, \lambda \to 0$.

We shall now formally map this problem to a zero temperature XY model with quenched phase shifts, or random Dzyaloshinskii-Moriya interactions [13–16] and related to dislocations in Bragg glasses [17], disordered solid films [18, 19] and glassy vortex phases in disordered type II superconductors in a transverse magnetic field (though there the interactions are often screened) [20, 21]. To do so, we note that although we started out with weak potential disorder $\sim \beta_{\rm o}\boldsymbol{\nabla}\phi_{\rm o}$, the gauge field $\mathcal{A}$ is no longer of a potential kind and is generally multiplicative in nature due to the nonlinear projection operator $\mathbb{P}$. As a consequence, $\mathcal{A}$ display finite correlations that survive even in the long wave-length limit ($q \to 0$). This essential feature becomes clear when explicitly writing

$$\mathcal{A}(\mathbf{r}) = -\frac{\beta_{\rm o}}{\lambda v_0^2}\,\hat{\mathbf{z}}\times[\boldsymbol{\nabla}\phi_{\rm o} - \boldsymbol{\nabla}\cdot(\hat{\mathbf{v}}\hat{\mathbf{v}}\;\phi_{\rm o}) + \phi_{\rm o}\;(\hat{\mathbf{v}}\cdot\boldsymbol{\nabla}\hat{\mathbf{v}})] = -\frac{\beta_{\rm o}}{\lambda v_0^2}\phi_{\rm o}(\mathbf{r})\,\hat{\mathbf{z}}\times(\hat{\mathbf{v}}\cdot\boldsymbol{\nabla}\hat{\mathbf{v}}) + \mathcal{O}(\boldsymbol{\nabla}), \tag{S15}$$

where the $\mathcal{O}(\boldsymbol{\nabla})$ terms are total derivatives. Computing the two-point correlator ($\overline{\mathcal{A}(\mathbf{r})} = \mathbf{0}$), we get

$$\overline{\mathcal{A}(\mathbf{r})\mathcal{A}(\mathbf{r}')} = \Phi_{\rm o}\frac{\beta_{\rm o}^2}{\lambda^2 v_0^4}\,\overline{\hat{\mathbf{v}}\hat{\mathbf{v}}|\partial_{||}\theta|^2}\,\delta(\mathbf{r}-\mathbf{r}') + \mathcal{O}(\nabla^2)\;. \tag{S16}$$

In general $\overline{\hat{\mathbf{v}}\hat{\mathbf{v}}|\partial_{||}\theta|^2}$ is a finite term. To compute it, we split $\theta(\mathbf{r}) = \delta\theta(\mathbf{r}) + \theta_v(\mathbf{r})$ into a smooth ($\delta\theta(\mathbf{r})$) and singular part ($\theta_v(\mathbf{r})$), so that

$$\oint_\Gamma \mathrm{d}\mathbf{s}\cdot\boldsymbol{\nabla}\theta_v = 2\pi\sum_i q_i\;, \tag{S17}$$

where the latter sum is over all the topological defects of charge $q_i = \pm 1$ (vortices and anti-vortices) enclosed by the contour $\Gamma$. Along with the charge density $\mathcal{C}(\mathbf{r}) = \sum_i q_i\delta(\mathbf{r}-\mathbf{r}_i)$, we have $\hat{\mathbf{z}}\cdot[\boldsymbol{\nabla}\times\boldsymbol{\nabla}\theta_v(\mathbf{r})] = 2\pi\mathcal{C}(\mathbf{r})$, while $\boldsymbol{\nabla}\times\boldsymbol{\nabla}\delta\theta(\mathbf{r}) = \mathbf{0}$. Therefore in Eq. S16, we perform the average over the smooth fluctuations $\delta\theta$ using the linearized theory (Eq. S12) and neglect any multiplicative corrections involving $\theta_v$ at lowest order, to get

$$\overline{\mathcal{A}(\mathbf{r})\mathcal{A}(\mathbf{r}')} \simeq \frac{\beta_{\rm o}^2\Phi_{\rm o}}{2\lambda^2 v_0^4}\,[M_+\mathbf{1} + M_-\boldsymbol{\sigma}_z]\,\delta(\mathbf{r}-\mathbf{r}') + \mathcal{O}(\nabla)\;, \tag{S18}$$

where $M_\pm = \overline{(\partial_x\delta\theta)^2} \pm \overline{\delta\theta^2(\partial_x\delta\theta)^2}$ within the linearized approximation, and $\boldsymbol{\sigma}_z$ is the third Pauli matrix. Both $M_\pm$ are positive constants $\propto \Phi_{\rm o}$ and are in general unequal, inheriting the global anisotropy of the polar ordered phase. As the linearized theory already predicts polar long-ranged order, we are primarily interested here in the topological sector. In other words, we only consider $\theta_v$ now, as $\delta\theta$ fluctuations are finite and can be effectively integrated out.

To analyze topological defects using the constraint from Eq. S14, we use the Parisi-Sourlas trick [22] to write

$$\mathcal{P}[\theta(\mathbf{r})] = \prod_{\mathbf{r}}\delta(\theta(\mathbf{r}) - \theta_{\phi_{\rm o}}(\mathbf{r})) = \prod_{\mathbf{r}}|\det(\mathcal{J})|\,\delta\left(\boldsymbol{\nabla}\theta - \mathcal{A}\right)\;, \tag{S19}$$

where $\theta_{\phi_{\rm o}}(\mathbf{r})$ refers to the solution of Eq. S14 as a parametric functional of the disorder realization $\phi_{\rm o}(\mathbf{r})$ and $\mathcal{J} = \boldsymbol{\nabla} - \delta\mathcal{A}/\delta\theta$ is the jacobian of the constraint. To lowest order, the correlations of $\mathcal{A}$ are set by the smooth fluctuations of $\theta$ and for now, we neglect the multiplicative dependence of $\mathcal{A}$ on $\theta_v$. The jacobian determinant in this limit is just a constant and can be neglected henceforth. Hence, integrating over the smooth fluctuations ($\delta\theta$), we get

$$\mathcal{P}[\theta_v(\mathbf{r})] \propto \prod_{\mathbf{r}}\delta(\boldsymbol{\nabla}\theta_v - \mathcal{A}_v) = \lim_{T\to 0}\prod_{\mathbf{r}}\sqrt{\frac{K}{2\pi T}}\;e^{-(K/2T)|\boldsymbol{\nabla}\theta_v - \mathcal{A}_v|^2}\;, \tag{S20}$$

where $\mathcal{A} = \boldsymbol{\nabla}a + \mathcal{A}_v$ (the smooth scalar $a$ can be absorbed into a shift of $\delta\theta$), such that $\boldsymbol{\nabla}\cdot\mathcal{A}_v = 0$ and $\hat{\mathbf{z}}\cdot(\boldsymbol{\nabla}\times\mathcal{A}_v) = Q$. We have additionally, used the Gaussian representation of the delta function and introduced an auxilliary temperature $T$, along with the elastic constant $K$ in the exponent for dimensional reasons as well as to make contact with a physical interpretation of orientational elasticity penalizing order parameter distortions. Hence we have an effective energy for the topological defect sector given by

$$E[\theta_v(\mathbf{r})] = -\lim_{T\to 0} T\ln\left(\mathcal{P}[\theta_v]\right) = \frac{K}{2}\int \mathrm{d}^2 r\;|\boldsymbol{\nabla}\theta_v - \mathcal{A}_v|^2\;, \tag{S21}$$

whose "zero temperature" ($T \to 0$) ground state controls the distribution of vortices in the active fluid. This completes our required mapping of the static defect distribution onto a zero temperature problem of a random 2D XY model. This formal mapping currently disregards any nonlinear fluctuation corrections that could nontrivially renormalize the elastic constant $K$ along with genuine nonequilibrium effects, and a fully detailed renormalization group treatment incorporating both is well beyond the current scope of this paper and will be presented elsewhere.

## VIII. DISORDER-INDUCED VORTEX CREATION AND ONSET OF MEANDERING FLOWS: A KOSTERLITZ-THOULESS STYLE ARGUMENT

We shall now use the effective energy in Eq. S21 to construct an argument for defect creation by balancing the elastic cost of creating an isolated vortex against the energy gained by virtue of its interaction with the background random charge $Q$. This is identical to arguments used in the equilibrium disordered context [14, 19] that have been supported by sophisticated functional renormalization group calculations as well [15, 16]. We first write the effective energy as a sum of an elastic term and a term arising from disorder (linear in $\mathcal{A}$), $E = E_{\rm el} + E_{\rm dis}$, with the $|\mathcal{A}|^2$ term providing only an irrelevant random constant. Given an isolated vortex centered at $\mathbf{r}_0$ with $\boldsymbol{\nabla}\theta_v = (\hat{\mathbf{z}} \times \hat{\mathbf{e}}_R)/R$ ($\mathbf{R} = \mathbf{r} - \mathbf{r}_0$), the effective elastic energy can be estimated to be

$$E_{\rm el} = \frac{K}{2}\int {\rm d}^2r |\boldsymbol{\nabla}\theta|^2 = \pi K \ln\left(\frac{L}{a}\right) \ , \tag{S22}$$

where $L$ is the system size and $a$ is the vortex core size (a microscopic cutoff). The effective energy gained due to the defect interaction with the disorder can be written as

$$E_{\rm dis}(\mathbf{r}_0) = K\int {\rm d}^2R\, \frac{\hat{\mathbf{e}}_R}{R} \times \mathcal{A}_v(\mathbf{R} + \mathbf{r}_0) = -K\int {\rm d}^2r \ln\left|\frac{\mathbf{r} - \mathbf{r}_0}{a}\right| Q(\mathbf{r}) \ , \tag{S23}$$

which has zero mean ($\overline{E_{\rm dis}(\mathbf{r}_0)} = 0$) and correlations

$$\overline{E_{\rm dis}(\mathbf{r}_0)^2} \simeq 2\pi K^2 \frac{\beta_{\rm o}^2 \Phi_{\rm o} M_+}{v_0^4\lambda^2} \ln\left(\frac{L}{a}\right) \ , \quad \overline{E_{\rm dis}(\mathbf{r}_0)E_{\rm dis}(\mathbf{r}_0')} \simeq 2\pi K^2 \frac{\beta_{\rm o}^2 \Phi_{\rm o} M_+}{v_0^4\lambda^2} \ln\left|\frac{\mathbf{r}_0 - \mathbf{r}_0'}{a}\right| \ . \tag{S24}$$

Within our simple approximation, the anisotropy of the gauge field correlator vanishes upon angular integration and only the isotropic component ($M_+$) contributes to the above expressions. This is sufficient for our scaling arguments. The typical gain in on-site energy from disorder is $\Delta = \left[\overline{E_{\rm dis}(\mathbf{r}_0)^2}\right]^{1/2} = K\Delta_0\sqrt{\ln(L/a)}$, where $\Delta_0 \simeq (\beta_{\rm o}/\lambda v_0^2)\sqrt{2\pi\Phi_{\rm o}M_+}$. Neglecting the long-ranged spatial correlations of $E_{\rm dis}$, this problem then maps onto the random energy model solved by Derrida [23]. While we have estimated the typical fluctuation of the disordered energy landscape, what really matters instead is the *optimum* energy gain from the disorder. Hence, the fluid can do better than just using the typical fluctuations of the impurities, but instead it can place a vortex at an optimal location so as to obtain a maximum energy gain from vortex screening with the random background charge to offset the elastic penalty of creating the vortex in the first place [14, 24]. For uncorrelated spatial sites, along with a Gaussian distribution of disorder, we can compute the following extreme value distribution for energy maxima,

$$P(E_{\rm max}) = \frac{\rm d}{{\rm d}E_{\rm max}}\left[\int_{-\infty}^{E_{\rm max}} {\rm d}E_{\rm dis}\, p(E_{\rm dis})\right]^N \ , \tag{S25}$$

with $N \sim (L/a)^2$ being the number of spatial sites to place a vortex and $p(E_{\rm dis}) = e^{-E_{\rm dis}^2/2\Delta^2}/\sqrt{2\pi\Delta^2}$ is the on-site distribution of disorder interaction energies. Using extreme value statistics, we find that $P(E_{\rm max})$ is peaked at its mean value given by $\overline{E_{\rm max}} \simeq \Delta\sqrt{2\ln(N)} = 2\Delta\sqrt{\ln(L/a)}$. Hence, including the maximum energy gain from the disorder, one finds that the ground state energy for an isolated vortex in a system of size $L$ is

$$E = \pi K\left[1 - \frac{2\Delta_0}{\pi}\right]\ln\left(\frac{L}{a}\right) \simeq \pi K\left[1 - \frac{\Phi_{\rm o}}{\Phi_c}\right]\ln\left(\frac{L}{a}\right) \ , \tag{S26}$$

where we have used the fact that $M_+ \propto \Phi_{\rm o}$ and $\Phi_c \sim \lambda v_0^2/\beta_{\rm o}$ is the transition threshold. Hence for $\Phi_{\rm o} > \Phi_c$, the probability of spontaneous vortex nucleation is one as $L/a \to \infty$, while for $\Phi_{\rm o} < \Phi_c$, this probability vanishes in the thermodynamic limit. So $\Phi_c$ is precisely the transition to the vortex glass phase seen in the experiment, and our theoretical argument through a mapping to the 2D random XY model rationalizes its existence.

We can additionally include the effect of a renormalized elastic stiffness that becomes scale dependent by virtue of nonlinear fluctuation corrections. At the simplest level, this corresponds to replacing $K$ by a logarithmic scale dependent average $\bar{K}_L$,

$$\bar{K}_L = \frac{1}{\ell_L}\int_0^{\ell_L} {\rm d}\ell\, K(\ell) \ , \tag{S27}$$

where $\ell = \ln(r/a)$ is a logarithmic spatial scale with $\ell_L = \ln(L/a)$ at the system size and $K(\ell)$ is the renormalized scale-dependent elastic constant. For a power law divergence of the elastic constant with distance $K(\ell) = K_0 e^{\mu\ell} = K_0(r/a)^\mu$, with an exponent $\mu > 0$, we have

$$\bar{K}_L = \frac{K_0}{\ln(L/a)} \int_1^{L/a} \frac{\mathrm{d}r}{r}\, r^\mu \simeq \frac{K_0}{\mu \ln(L/a)} \left(\frac{L}{a}\right)^\mu , \tag{S28}$$

for $L \gg a$. As a result, for a power law scale dependent elastic stiffness, we can rewrite the ground state energy from Eq. S26 now as

$$E \simeq \frac{\pi K_0}{\mu} \left[1 - \frac{\Phi_\mathrm{o}}{\Phi_c}\right] \left(\frac{L}{a}\right)^\mu . \tag{S29}$$

Hence within this picture of disorder induced vortex creation, nonequilibrium activity enters in two places-the first is in converting the random potential disorder into a random backgroundgauge field and charge by balancing density fluxes with convective fluxes; and the second is in a possible scale dependence of the defect interaction through a renormalized stiffnes. Note that, while the existence of the transition at $\Phi_\mathrm{o} = \Phi_c$ remains unchanged by a nontrivial $K(\ell)$, spatial correlations and dynamic features are expected to strongly depend on $\mu$ and $K(\ell)$ in general, as evidenced even in equilibrium systems with long-ranged defect interactions [25].

## IX. DESCRIPTION OF THE SUPPLEMENTARY VIDEOS

**Supplementary Video 1:** Flocking motion emerges in an ensemble of half a million colloidal rollers. The circular chamber has a diameter of 6 mm and includes no obstacle. When the DC electric field is turned on, the rollers start propelling along random directions. After a short transient, they self-organize into a polar fluid. The polar-fluid flow self-organizes to form a steady macroscopic vortex. Colloid area fraction $\rho_0 = 0.25$. Colloid diameter: $4.8\,\mu$m. Field amplitude: $E_0 = 4.5\,\mathrm{V}/\mu$m. Video recorded at 190 fps, played at 50 fps.

**Supplementary Video 2:** Coarsening dynamics of the polar flows in a 3 mm wide circular chamber including no obstacle. The movie shows the Schlieren texture and the corresponding instantaneous velocity field. The dots indicate the position of the $\pm1$ topological defects. Colloid fraction $\rho_0 = 0.08$. PIV box size: $76.5\,\mu$m. Field amplitude: $E_0 = 4.5\,\mathrm{V}/\mu$m. Video recorded at 190 fps, played at 50 fps.

**Supplementary Video 3:** Close-up movie on a collection of colloidal rollers (dark) propelling though lithographied obstacles (light patterns). The center of the cylindrical obstacles of diameter $10\,\mu$m are placed at random and may overlap. The lithographied obstacles repel the rollers at a finite distance, but leave their speed unaltered. Obstacle fraction: $\Phi_\mathrm{o} = 15\,\%$. Colloid fraction $\rho_0 = 0.08$. Colloid diameter: $4.8\,\mu$m. Field amplitude: $E_0 = 4.5\,\mathrm{V}/\mu$m. Video recorded at 190 fps, played at 25 fps.

**Supplementary Video 4:** A polar liquid flows through a 3 mm wide circular chamber including a random lattice of obstacles (highlighted in orange). At small disorder, the obstacles hardly alter the coarsening dynamics of the polar liquids. The spontaneous flows self-organize into a macroscopic vortex over system-spanning scales. Obstacle fraction: $\Phi_\mathrm{o} = 3\,\%$. Colloid fraction $\rho_0 = 0.08$. Colloid diameter: $4.8\,\mu$m. Field amplitude: $E_0 = 4.5\,\mathrm{V}/\mu$m. Video recorded at 190 fps, played at 25 fps.

**Supplementary Video 5:** Meandering patterns formed when a collection of Quincke rollers propel through a random lattice of obstacles (pink color). The vortex structure observed in a pure system is detroyed but local order subsists. Obstacle fraction: $\Phi_\mathrm{o} = 15\,\%$. Colloid fraction $\rho_0 = 0.08$. Chamber diameter: 3 mm. Colloid diameter: $4.8\,\mu$m. Field amplitude: $E_0 = 4.5\,\mathrm{V}/\mu$m. Video recorded at 190 fps, played at 25 fps.

**Supplementary Video 6:** A dense lattices of obstacles (blue color) suppresses the emergence of collective motion. The colloidal rollers form an active-gas phase. Obstacle fraction: $\Phi_\mathrm{o} = 36\,\%$. Colloid fraction $\rho_0 = 0.08$. Chamber diameter: 3 mm. Colloid diameter: $4.8\,\mu$m. Field amplitude: $E_0 = 4.5\,\mathrm{V}/\mu$m. Video recorded at 190 fps, played at 25 fps.

**Supplementary Video 7:** Flocking through a periodic lattice of obstacles (orange color). A polar liquid emerges and forms a robust vortex pattern merely deformed by the underlying lattice geometry. Obstacle fraction: $\Phi_\mathrm{o} = 15\,\%$.

Chamber diameter: 3 mm. Colloid fraction $\rho_0 = 0.08$. Colloid diameter: 4.8 $\mu$m. Field amplitude: $E_0 = 4.5\,\mathrm{V}/\mu\mathrm{m}$. Video recorded at 190 fps, played at 25 fps.

---


[1] Peter J Lu, Peter A Sims, Hidekazu Oki, James B Macarthur, and David A Weitz, "Target-locking acquisition with real-time confocal (tarc) microscopy," Optics express **15**, 8702–8712 (2007).

[2] John C Crocker and David G Grier, "Methods of digital video microscopy for colloidal studies," Journal of colloid and interface science **179**, 298–310 (1996).

[3] D. Blair and E. Dufresne, "The matlab particle tracking code repository," .

[4] John Toner, Yuhai Tu, and Sriram Ramaswamy, "Hydrodynamics and phases of flocks," Annals of Physics **318**, 170 – 244 (2005), special Issue.

[5] M. C. Marchetti, J. F. Joanny, S. Ramaswamy, T. B. Liverpool, J. Prost, Madan Rao, and R. Aditi Simha, "Hydrodynamics of soft active matter," Rev. Mod. Phys. **85**, 1143–1189 (2013).

[6] Delphine Geyer, Alexandre Morin, and Denis Bartolo, "Sounds and hydrodynamics of polar active fluids," Nature materials **17**, 789 (2018).

[7] John Toner, Nicholas Guttenberg, and Yuhai Tu, "Swarming in the dirt: Ordered flocks with quenched disorder," Phys. Rev. Lett. **121**, 248002 (2018).

[8] John Toner, Nicholas Guttenberg, and Yuhai Tu, "Hydrodynamic theory of flocking in the presence of quenched disorder," Phys. Rev. E **98**, 062604 (2018).

[9] Alexandre Morin, Nicolas Desreumaux, Jean-Baptiste Caussin, and Denis Bartolo, "Distortion and destruction of colloidal flocks in disordered environments," Nature Physics **13**, 63 (2017).

[10] Rakesh Das, Manoranjan Kumar, and Shradha Mishra, "Polar flock in the presence of random quenched rotators," Phys. Rev. E **98**, 060602 (2018).

[11] Ananyo Maitra, "Active uniaxially ordered suspensions on disordered substrates," arXiv preprint arXiv:1910.07334 (2019), 10.1103/PhysRevE.101.012605.

[12] Oleksandr Chepizhko, Eduardo G. Altmann, and Fernando Peruani, "Optimal noise maximizes collective motion in heterogeneous media," Phys. Rev. Lett. **110**, 238101 (2013).

[13] Michael Rubinstein, Boris Shraiman, and David R Nelson, "Two-dimensional xy magnets with random dzyaloshinskii-moriya interactions," Physical Review B **27**, 1800 (1983).

[14] Thomas Nattermann, Stefan Scheidl, Sergey E Korshunov, and Mai Suan Li, "Absence of reentrance in the two-dimensional xy-model with random phase shift," Journal de Physique I **5**, 565–572 (1995).

[15] David Carpentier and Pierre Le Doussal, "Disordered xy models and coulomb gases: renormalization via traveling waves," Physical review letters **81**, 2558 (1998).

[16] David Carpentier and Pierre Le Doussal, "Topological transitions and freezing in xy models and coulomb gases with quenched disorder: renormalization via traveling waves," Nuclear Physics B **588**, 565–629 (2000).

[17] Pierre Le Doussal and Thierry Giamarchi, "Dislocations and bragg glasses in two dimensions," Physica C: Superconductivity **331**, 233–240 (2000).

[18] David R Nelson, "Reentrant melting in solid films with quenched random impurities," Physical Review B **27**, 2902 (1983).

[19] Min-Chul Cha and HA Fertig, "Disorder-induced phase transitions in two-dimensional crystals," Physical review letters **74**, 4867 (1995).

[20] Matthew P. A. Fisher, "Vortex-glass superconductivity: A possible new phase in bulk high-$t_c$ oxides," Phys. Rev. Lett. **62**, 1415–1418 (1989).

[21] Thomas Nattermann and Stefan Scheidl, "Vortex-glass phases in type-ii superconductors," Advances in Physics **49**, 607–704 (2000).

[22] Giorgio Parisi and Nicolas Sourlas, "Random magnetic fields, supersymmetry, and negative dimensions," Physical Review Letters **43**, 744 (1979).

[23] Bernard Derrida, "Random-energy model: An exactly solvable model of disordered systems," Physical Review B **24**, 2613 (1981).

[24] SE Korshunov and Thomas Nattermann, "Phase diagram of a josephson junction array with positional disorder," Physica B: Condensed Matter **222**, 280–286 (1996).

[25] JM Kosterlitz, "Phase transitions in long-range ferromagnetic chains," Physical Review Letters **37**, 1577 (1976).
